# Supplementary material for: Cavity Quantum Electrodynamics Ring Coupled Cluster and the Random Phase Approximation
Source: arXiv:2602.09968 ancillary file (2026-04-09)
Supplement: Supplementary file 1 [file qed_rpa_si.pdf]

# Supporting Information for: Cavity Quantum Electrodynamics Ring Coupled Cluster and the Random Phase Approximation

A. Eugene DePrince III,[1, a)] Stephen H. Yuwono,[1] and Henk Eshuis[2]

[1)] *Department of Chemistry and Biochemistry, Florida State University, Tallahassee, FL 32306-4390 USA*

[2)] *Department of Chemistry and Biochemistry, Montclair State University, Montclair, New Jersey 07043, USA*

[a)] Electronic mail: adeprince@fsu.edu

The residual equations for the quantum electrodynamics (QED) coupled-cluster doubles (CCD) approach are

$$\langle \Phi_{ij}^{ab} | \langle 0_\text{p} | \bar{H} | 0_\text{p} \rangle | 0_\text{e} \rangle = 0 \tag{S1}$$

$$\langle \Phi_{i}^{a} | \langle 1_\text{p} | \bar{H} | 0_\text{p} \rangle | 0_\text{e} \rangle = 0 \tag{S2}$$

$$\langle 0_\text{e} | \langle 2_\text{p} | \bar{H} | 0_\text{p} \rangle | 0_\text{e} \rangle = 0 \tag{S3}$$

Explicit, programmable expressions for these residual equations are

$$\begin{aligned}
0 =& -P(i,j)P(a,b)\sqrt{\frac{\omega_\text{cav}}{2}}d_{ai}\ {}^{[1]}t_j^b - P(i,j)P(a,b)\sqrt{\frac{\omega_\text{cav}}{2}}d_{kc}t_{ki}^{ca}\ {}^{[1]}t_j^b \\
& - P(a,b)\sqrt{\frac{\omega_\text{cav}}{2}}d_{kc}t_{ij}^{ca}\ {}^{[1]}t_k^b - P(i,j)\sqrt{\frac{\omega_\text{cav}}{2}}d_{kc}t_{jk}^{ab}\ {}^{[1]}t_i^c \\
& - P(i,j)f_j^k t_{ik}^{ab} + P(a,b)f_c^a t_{ij}^{cb} + \langle ab||ij\rangle + \frac{1}{2}\langle kl||ij\rangle t_{kl}^{ab} \\
& + P(i,j)P(a,b)\langle ka||ci\rangle t_{kj}^{cb} + \frac{1}{2}\langle ab||cd\rangle t_{ij}^{cd} - \frac{1}{2}P(i,j)\langle kl||cd\rangle t_{ik}^{ab}t_{jl}^{cd} + \frac{1}{4}\langle kl||cd\rangle t_{kl}^{ab}t_{ij}^{cd} \\
& - \frac{1}{2}\langle kl||cd\rangle t_{kl}^{ca}t_{ij}^{db} + P(i,j)\langle kl||cd\rangle t_{jl}^{ca}t_{ik}^{db} - \frac{1}{2}\langle kl||cd\rangle t_{ij}^{ca}t_{kl}^{db}
\end{aligned} \tag{S4}$$

$$\begin{aligned}
0 =&\ {}^{[1]}t_i^a\omega_\text{cav} - \sqrt{\frac{\omega_\text{cav}}{2}}d_{ai} - \sqrt{\frac{\omega_\text{cav}}{2}}d_{jb}t_{ij}^{ab} - \sqrt{\frac{\omega_\text{cav}}{2}}d_{ai}\ {}^{[2]}t \\
& - \sqrt{\frac{\omega_\text{cav}}{2}}d_{jb}t_{ij}^{ab}\ {}^{[2]}t - \sqrt{\frac{\omega_\text{cav}}{2}}d_{jb}\ {}^{[1]}t_i^a\ {}^{[1]}t_j^b + 2\sqrt{\frac{\omega_\text{cav}}{2}}d_{jb}\ {}^{[1]}t_j^a\ {}^{[1]}t_i^b - f_i^j\ {}^{[1]}t_j^a \\
& + f_b^a\ {}^{[1]}t_i^b + \langle ja||bi\rangle\ {}^{[1]}t_j^b - \frac{1}{2}\langle kj||bc\rangle t_{ij}^{bc}\ {}^{[1]}t_k^a - \frac{1}{2}\langle kj||bc\rangle t_{kj}^{ba}\ {}^{[1]}t_i^c \\
& + \langle kj||bc\rangle t_{ij}^{ba}\ {}^{[1]}t_k^c
\end{aligned} \tag{S5}$$

$$0 = 2\ {}^{[2]}t\,\omega_\text{cav} - 2\sqrt{\frac{\omega_\text{cav}}{2}}d_{ia}\ {}^{[1]}t_i^a - 2\sqrt{\frac{\omega_\text{cav}}{2}}d_{ia}\ {}^{[1]}t_i^a\ {}^{[2]}t + \langle ij||ab\rangle\ {}^{[1]}t_i^a\ {}^{[1]}t_j^b \tag{S6}$$

respectively. Note that all antisymmetrized electron repulsion integral terms are dressed to include dipole self-energy contributions, *i.e.*

$$\langle pq||rs\rangle \rightarrow \langle pq||rs\rangle + d_{pr}d_{qs} - d_{ps}d_{qr} \tag{S7}$$

The symbol $d_{pq}$ represents a dressed dipole integral, which is defined in the main text. $P(i,j)$ and $P(a,b)$ are permutation operators, *e.g.*, $P(i,j)A_i^aB_j^b = A_i^aB_j^b - A_j^aB_i^b$. These equations were adapted from residual equations generated by the $\texttt{p}^\dagger\texttt{q}$ package. Note that the definition of the double photon creation operator in $\texttt{p}^\dagger\texttt{q}$ differs from that used in this work by a factor of two. These equations use the definition in the main text.

Given the residual equations above, the ring simplifications can be obtained in the following way. First, we transpose all doubles amplitudes so that the labels $a/i$, $b/j$, $c/k$, and $d/l$ are paired, and we define

$$T^{2,0}_{ai,bj} = {}^{[0]}t^{ab}_{ij} \tag{S8}$$

$$T^{1,1}_{ai} = {}^{[1]}t^{a}_{i} \tag{S9}$$

$$T^{0,2} = {}^{[2]}t \tag{S10}$$

Second, we eliminate any permutations that break such pairings. Third, we discard any contractions that do not correspond to familiar ring-type particle-hole contractions in the electronic space or electron-photon ring contractions corresponding to electron excitation / photon annihilation or photon creation / electron de-excitation. The ring simplifications of these residual equations are then

$$0 = \langle ab||ij\rangle + T^{2,0}_{ai,jb}(\varepsilon_a+\varepsilon_b-\varepsilon_i-\varepsilon_j) + \sum_{ck}\langle ic||ak\rangle T^{2,0}_{ck,bj} + \sum_{ck}\langle kb||cj\rangle T^{2,0}_{ai,ck} + \sum_{cdkl} T^{2,0}_{ai,ck}\langle kl||cd\rangle T^{2,0}_{dl,bj}$$
$$-\sqrt{\frac{\omega_{\text{cav}}}{2}}\sum_{ck} T^{2,0}_{ai,ck} d_{ck} T^{1,1}_{bj} - \sqrt{\frac{\omega_{\text{cav}}}{2}} T^{1,1}_{ai}\sum_{ck} d_{ck} T^{2,0}_{ck,bj} - \sqrt{\frac{\omega_{\text{cav}}}{2}} T^{1,1}_{ai} d_{bj} - \sqrt{\frac{\omega_{\text{cav}}}{2}} d_{ai} T^{1,1}_{bj} \tag{S11}$$

$$0 = -\sqrt{\frac{\omega_{\text{cav}}}{2}} d_{ai} + T^{1,1}_{ai}\omega_{\text{cav}} + (\varepsilon_a-\varepsilon_i)T^{1,1}_{ai} + \sum_{bj}\langle ib||aj\rangle T^{1,1}_{bj} + \sum_{bckj} T^{1,1}_{ck} T^{2,0}_{ai,bj}\langle jk||bc\rangle$$
$$-\sqrt{\frac{\omega_{\text{cav}}}{2}}\sum_{bj} T^{2,0}_{ai,bj} d_{bj} - \sqrt{\frac{\omega_{\text{cav}}}{2}} T^{1,1}_{ai}\sum_{bj} d_{bj} T^{1,1}_{bj} - \sqrt{\frac{\omega_{\text{cav}}}{2}} d_{ai} T^{0,2} - \sqrt{\frac{\omega_{\text{cav}}}{2}} T^{0,2}\sum_{bj} T^{2,0}_{ai,bj} d_{bj} \tag{S12}$$

and

$$0 = 2\omega_{\text{cav}} T^{0,2} - 2\sqrt{\frac{\omega_{\text{cav}}}{2}} T^{0,2}\sum_{ai} d_{ai} T^{1,1}_{ai} - 2\sqrt{\frac{\omega_{\text{cav}}}{2}}\sum_{ai} d_{ai} T^{1,1}_{ai} + \sum_{abij}\langle ij||ab\rangle T^{1,1}_{ai} T^{1,1}_{bj} \tag{S13}$$

respectively.

Table S1 provides differences in correlation energies obtained from QED-drCCD and QED-dRPA at different coupling strengths ($\lambda$, given in a.u.) for a water molecule (described by the cc-pVDZ basis set) embedded within a single-mode optical cavity. The O–H bond length is fixed at 1 Å, the H–O–H bond angle is fixed at 104.5°, and the molecule is oriented such that the principal rotation axis is aligned along the $z$ direction. The molecule is coupled to a $z$-polarized

single-mode optical cavity with a fundamental frequency of 0.415668 $E_h$, which is resonant with the lowest-energy excited state of the molecule with a non-zero transition moment along the $z$ direction (computed at the RPA/cc-pVDZ level, in the absence of the cavity). Table S1 also quantifies the influence of the photon-photon channel by providing the difference between ground-state correlation energies obtained from a QED-drCCD model that ignores $T^{0,2}$ in the cluster operator and the full QED-drCCD approach.

| $\lambda$ | $E_c^{dRPA}$ | $E_c^{drCCD}$ | $T^{0,2}$ channel |
|---|---|---|---|
| 0.00 | -0.23345931 | -0.23345931 | 0.00000000 |
| 0.01 | -0.23350803 | -0.23350803 | 0.00000000 |
| 0.02 | -0.23365413 | -0.23365413 | 0.00000003 |
| 0.03 | -0.23389754 | -0.23389754 | 0.00000014 |
| 0.04 | -0.23423807 | -0.23423807 | 0.00000046 |
| 0.05 | -0.23467551 | -0.23467551 | 0.00000111 |
| 0.10 | -0.23830469 | -0.23830469 | 0.00001683 |
| 0.20 | -0.25259114 | -0.25259114 | 0.00022470 |
| 0.30 | -0.27589557 | -0.27589557 | 0.00088002 |
| 0.40 | -0.30799274 | -0.30799274 | 0.00207037 |
| 0.50 | -0.34871719 | -0.34871719 | 0.00370901 |

TABLE S1. The correlation energies obtained from QED-drCCD and QED-dRPA and the change in the correlation energy when ignoring the $T^{0,2}$ channel ($E_h$).
